# Supplementary material for: Appearance of T$_d^*$ phase across the T$_{d}$-1T$^{\prime}$ phase boundary in Weyl semimetal MoTe$_{2}$
Source: arXiv:1902.06799 source file (2019-08-26)
Supplement: Supplementary file 1 [file Supplemental.pdf]

# Supplemental Materials: Appearance of $T_d^*$ phase across the $T_d$–1T′ phase boundary in Weyl semimetal $MoTe_2$

Yu Tao,[1] John A. Schneeloch,[1] Chunruo Duan,[1] Masaaki Matsuda,[2] Sachith E. Dissanayake,[2,*] Adam A. Aczel,[2,3] Jaime A. Fernandez-Baca,[2] Feng Ye,[2] and Despina Louca[1,†]

[1]*Department of Physics, University of Virginia, Charlottesville, Virginia 22904, USA*
[2]*Neutron Scattering Division, Oak Ridge National Laboratory, Oak Ridge, Tennessee 37831, USA*
[3]*Department of Physics and Astronomy, University of Tennessee, Knoxville, Tennessee 37996, USA*

## CRYSTAL GROWTH DETAILS

The $MoTe_2$ crystals measured in this work include "MT1", which was measured with neutrons, and two used in resistance measurements that were grown similarly as for MT1. The "MT2" crystal, also measured with neutrons, had a composition of $Mo_{1-x}W_xTe_2$ with $x \lesssim 0.01$.

Elemental powders were mixed, pressed into a pellet, sealed into an evacuated silica ampoule, and sintered at 950 °C for 7 to 29 hours before quenching in liquid nitrogen or water. For MT1, the sintered material $MoTe_{2.1}$ was combined with Te in a 1:3 mass ratio and cooled from 1150 °C to 950 °C in 500 h. For MT2, the initial sintered material was $Mo_{0.8}W_{0.2}Te_2$, though energy-dispersive X-ray spectroscopy (EDS) showed the W-fraction ($x$ in $Mo_{1-x}W_xTe_2$) of the grown crystal to be $x \lesssim 0.01$. (Specifically, in MT2, 15 of 18 EDS measurements showed no W-fraction, while the other 3 measurements showed values of $x$ of 0.012, 0.015, and 0.018.) The sintered mass was combined with Te in a 2:1 mass ratio, heated to 1250 °C, and cooled to 950 °C in 70 h. (We speculate that the low W-substitution of MT2 was related to the high growth temperature of 1250 °C. For cooling from 1150 °C, we have grown $Mo_{1-x}W_xTe_2$ crystals with $x$ up to ∼0.5, which will be the subject of a future paper.) Both the MT1 and MT2 crystals were quenched at 950 °C in liquid nitrogen or water. Excess Te was decanted in a post-annealing step at ∼1000 °C, then quenched in water. For both crystals, EDS showed roughly stoichiometric molar ratios of Te to the metal elements, 2.05(17):1 for MT1 and 1.96(2):1 for MT2. The out-of-plane component of the $c$-axis lattice constant, $c_o$, is known to increase with W-substitution, by roughly 0.003 Å per percent increase in $x$ [1]; however, we measured no difference in $c_o$ between our crystals, with 13.775(3) Å for MT1 and 13.774(5) Å for MT2 as determined by longitudinal neutron scattering scans along the (004) Bragg peak on CG4C and HB1A, respectively, agreeing with the low W-doping level of MT2 found via EDS.

* Present address: Duke University, Dept. of Physics, Durham, NC 27708
† Corresponding author. Email: louca@virginia.edu

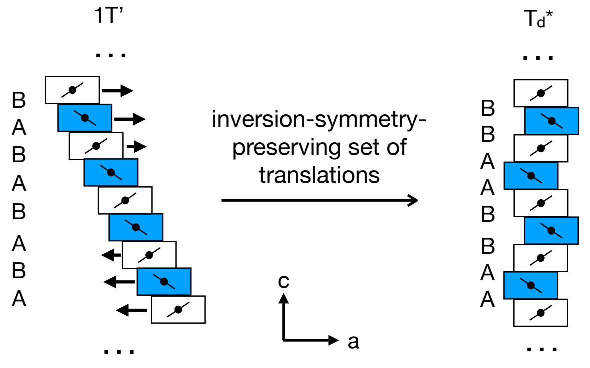


FIG. S1. Illustration of the set of inversion-symmetry-preserving translations that map 1T′ to $T_d^*$.

## CENTROSYMMETRY OF $T_d^*$

Here, we explain how the AABB-stacking proposed for $T_d^*$ should be centrosymmetric, since it can be constructed by applying a centrosymmetric series of translations to the centrosymmetric 1T′ structure. The process is depicted in Fig. S1.

Starting from the ...ABABABAB... stacking of 1T′, we leave one layer fixed before applying translations. In 1T′, every layer has centers of inversion symmetry, so any layer can be chosen to be fixed. Next, let $i$ denote the $i$th nearest neighboring layer from the fixed layer, either above or below as specified. Let us use the word "flipped" to denote either A→B or B→A transformations. The transformation that maps 1T′ to $T_d^*$ is as follows: Both above and below the fixed layer, flip $i = 2 + 4n$ and $i = 3 + 4n$ for every integer $n \geq 0$.

In more detail, an A→B or B→A operation applied to a given layer results in a translation applied to every layer to the outside of the given layer (with "outside" defined relative to the fixed layer). The direction of the translation of A→B alternates layer-by-layer, and, for a given layer, is opposite that of B→A.

Because every A→B operation is balanced by a B→A operation on the opposite side of, and equal distance from, the fixed layer, the total sequence of translations mapping 1T′ to $T_d^*$ preserves inversion symmetry. Thus, if $T_d^*$ has the AABB stacking (as we argue in the main text), it should be centrosymmetric. In principle, sponta-

neous symmetry breaking is possible, but the layers hosting centers of inversion symmetry in $T_d^*$ (between neighboring A- and B-type interlayer boundaries) have neighboring layers in a similar position as for 1T′, for which inversion symmetry breaking has not been reported. Also, theoretical calculations suggest individual layers tend toward inversion symmetry [2].

## REFINEMENT OF THE $T_d^*$ STRUCTURE FROM CORELLI DATA

Refinement of single crystal neutron scattering data was performed to determine the coordinates of the $T_d^*$ structure. The neutron scattering data were taken on the MT1 crystal at CORELLI, and the data taken on warming to 300 K were used in the refinement. An orientation matrix (a.k.a. UB matrix) of the main phase was determined by manually indexing its major Bragg reflections. The scattering data were normalized by the incoming flux, then positions were converted into reciprocal lattice coordinates using the UB matrix after subtracting the background from the sample holder and the thermal shielding. Since the sample exhibits phase coexistent during the phase transition, obtaining the structure factors of a certain phase required knowing the volume fractions of each phase and each twin structure, which was done by fitting the normalized data with the calculated scattering patterns for each phase and each twin based on their ideal structures. The obtained volume fractions for each temperature are shown in Fig. S2(c). The fitting was done using peaks within $-1 \le H \le 8$, $-1 \le K \le 1$, $-20 \le L \le 20$. (The lattice parameters were not refined, as is typical in single-crystal diffraction.) Refinement was done assuming $P2_1/m$ symmetry, the highest possible for a structure built with AABB stacking, and used the 131 reflections that were strong enough to be integrated and used in the refinement. Another symmetry, $P2_1$, was attempted, but refinement with this symmetry led to excessive peak intensities at Bragg peak locations not included in the refinement due to being too weak. The refinement resulted in $R_w = 0.13$. The refined positions are listed in Table S1.

TABLE S1. Refined atomic positions in the $T_d^*$ phase using the $P2_1/m$ space group. The MT1 crystal was measured in CORELLI on warming to 300 K. The lattice constants were $a$ = 6.33 Å, $b$ = 3.48 Å, $c$ = 27.66 Å, and $\beta$ =∼90°. The $\chi^2$ of the refinement was 5.8, and $R_w$ was 0.13. The $U_{iso}$ parameters were -0.002(5) for Mo and 0.002(4) for Te.

| atom | $x$ | $y$ | $z$ | atom | $x$ | $y$ | $z$ |
|---|---|---|---|---|---|---|---|
| Mo1 | 0.71(2) | 0.75 | 0.995(4) | Mo2 | 0.91(2) | 0.25 | 0.250(3) |
| Mo3 | 0.33(1) | 0.25 | 0.491(3) | Mo4 | 0.22(2) | 0.75 | 0.253(4) |
| Te1 | 0.06(2) | 0.75 | 0.054(5) | Te2 | 0.47(2) | 0.25 | 0.308(4) |
| Te3 | 0.58(2) | 0.25 | 0.074(5) | Te4 | 0.01(2) | 0.75 | 0.322(4) |
| Te5 | 0.16(2) | 0.25 | 0.170(4) | Te6 | 0.40(2) | 0.75 | 0.429(5) |
| Te7 | 0.64(2) | 0.75 | 0.199(4) | Te8 | 0.92(1) | 0.25 | 0.452(3) |

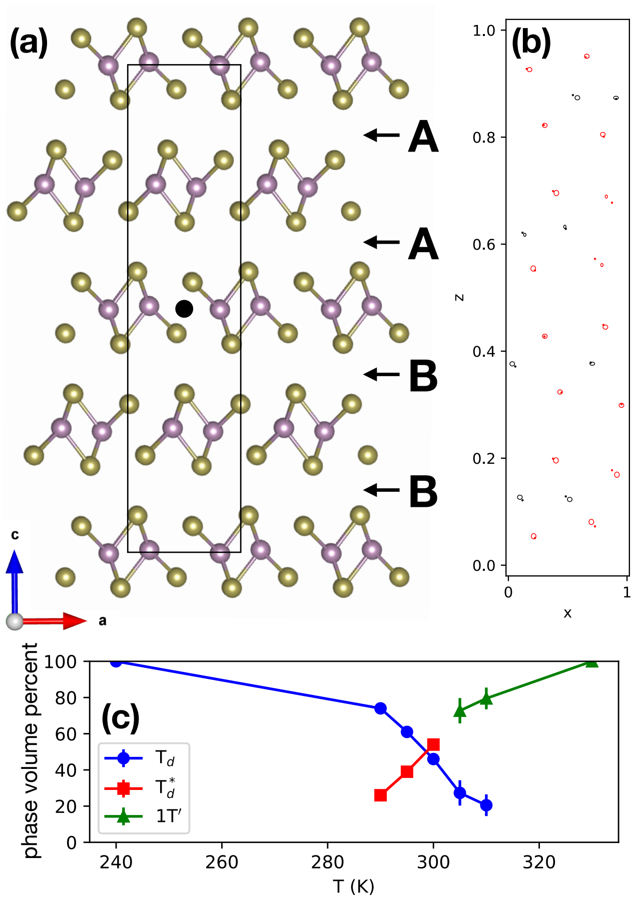


FIG. S2. (a) Proposed crystal structure of the $T_d^*$ phase in the $a$-$c$ plane, based on an "AABB" stacking pattern. "A" and "B" denote boundaries formed by the A/B stacking operations as described in the main text. Image of atomic coordinates generated by VESTA [5]. Gold and purple balls are Mo and Te atoms, respectively. The dot shows an inversion symmetry center. (b) A comparison between fitted positions in the $x$-$z$ plane (along the $a$- and $c$-directions) and "ideal" positions generated by the AABB stacking. The ideal positions are dots, and the fitted positions are ellipses, with the heights and widths of the ellipses being twice the $x$- and $z$-position uncertainties given in Table S1. (c) Volume fractions of the $T_d$, $T_d^*$, and 1T′ phases derived from fitting to the CORELLI data on MT1.

Figure S2(b) shows a comparison between the refined positions and "ideal" positions (i.e., from a structure constructed by an AABB stacking of layers with the $T_d$-phase coordinates reported in Ref. [3]), where ideal positions are plotted as dots and the refined positions are plotted as ellipses with heights and widths given by twice the uncertainties listed in Table S1. There is some deviation between the fitted and ideal positions, which would result in visible peaks in the $0KL$ plane at non-even $K+L$ (e.g., $(0, 1, 6.5)$ would have an intensity of ∼16% that of the (002) peak), in contrast to the lack of visible non-

even $K+L$ peaks in the $0KL$ plane in our data. Thus, the ideal coordinates from the AABB stacking model are likely to be closer to the true $T_d^*$ structure than the refined coordinates. (In principle, we would expect some intensity at non-even $K+L$ peaks due to the $P2_1/m$ symmetry not requiring the exact same $c$-axis intralayer coordinates for each layer. We can estimate this intensity by comparison with 1T′, which should also have nonzero intensity at odd $K+L$ $0KL$ peaks for the same reason. Given the 1T′ coordinates in Ref. [4], the maximum intensity of an odd $K+L$ peak in the $0KL$ plane within $-1 \leq K \leq 1$ and $-11 \leq L \leq 11$ is at $(0,1,10)$, having ∼0.08% of the intensity at (002). We would not expect peaks this weak to be visible in Fig. 2(a-f) in the main text.)

## DIFFUSE SCATTERING CHANGES WITH WARMING AND COOLING

In Fig. S3, we plot intensity along $(2,0,L)$ at a number of selected temperatures for MT2 (from the same data set used for Fig. 1(d) and 1(e)), focusing on the diffuse scattering near $L = 2.5$. We see that, as the $T_d$ and 1T′ Bragg peak intensities increase on heating or cooling toward the temperature extremes in Fig. 3(a,b), the diffuse scattering decreases concomitantly. On the other hand, on heating from $T_d$ or cooling from 1T′, no change is seen in the diffuse scattering until an onset temperature is passed (∼280 K on cooling from 1T′, and ∼260 K on warming from $T_d$.)

## LONG HYSTERESIS TAIL IN RESISTIVITY

In Fig. S4(a), we show resistivity data taken through a hysteresis loop from 300 K to 2 K and back to 300 K. A long tail in the hysteresis persists to low temperature. Fig. S4(b) plots the difference between the cooling and warming resistivity data, showing that the hysteresis persists down to at least 50 K. In the main text, we argue that the residual hysteresis in these resistivity data (as well as data reported in the literature, e.g., Ref. [6]) and the residual hysteresis in diffuse scattering and Bragg peak intensities likely have a similar cause, which we speculate to be changes in the presence of 1T′ and $T_d$ twin boundaries.


[1] S. M. Oliver, R. Beams, S. Krylyuk, I. Kalish, A. K. Singh, A. Bruma, F. Tavazza, J. Joshi, I. R. Stone, S. J. Stranick, A. V. Davydov, and P. M. Vora, "The structural phases and vibrational properties of $Mo_{1-x}W_xTe_2$ alloys," 2D Mater. **4**, 045008 (2017).

[2] C. Heikes, I-L. Liu, T. Metz, C. Eckberg, P. Neves, Y. Wu, L. Hung, P. Piccoli, H. Cao, J. Leao, J. Paglione, T. Yildirim, N. P. Butch, and W. Ratcliff, "Mechanical control of crystal symmetry and superconductivity in Weyl semimetal $MoTe_2$," Phys. Rev. Mater. **2**, 074202 (2018).

[3] Y. Qi, P. G. Naumov, M. N. Ali, C. R. Rajamathi, W. Schnelle, O. Barkalov, M. Hanfland, S.-C. Wu, C. Shekhar, Y. Sun, V. Süß, M. Schmidt, U. Schwarz, E. Pippel, P. Werner, R. Hillebrand, T. Förster, E. Kampert, S. Parkin, R. J. Cava, C. Felser, B. Yan, and S. A. Medvedev, "Superconductivity in Weyl semimetal candidate $MoTe_2$," Nat. Commun. **7**, 11038 (2016).

[4] B. E. Brown, "The crystal structures of $WTe_2$ and high-temperature $MoTe_2$," Acta Crystallogr. **20**, 268–274 (1966).

[5] K. Momma and F. Izumi, "VESTA 3 for three-dimensional visualization of crystal, volumetric and morphology data," J. Appl. Crystallogr. **44**, 1272–1276 (2011).

[6] T. Zandt, H. Dwelk, C. Janowitz, and R. Manzke, "Quadratic temperature dependence up to 50 K of the resistivity of metallic $MoTe_2$," J. Alloys Compd. Proceedings of the 15th International Conference on Solid Compounds of Transition Elements, **442**, 216–218 (2007).

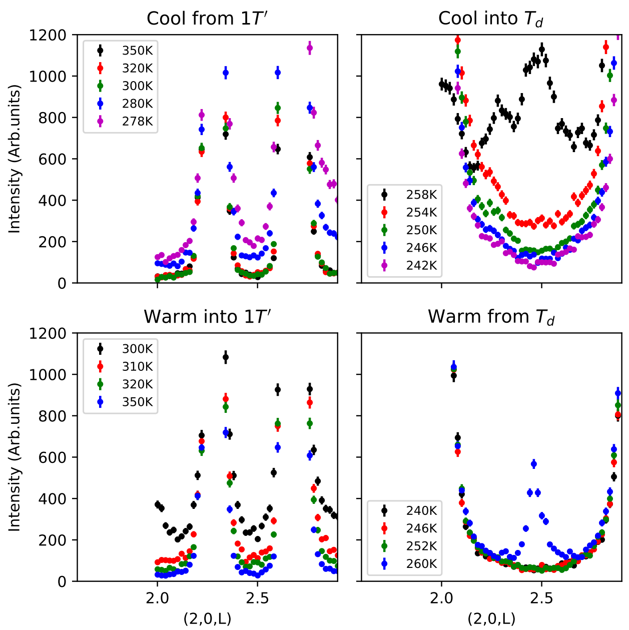


FIG. S3. Diffuse scattering intensity around (2,0,2.5) when cooling or warming to and from the extremes of the $T_d$ and 1T′ phases for MT2 at various temperatures. Data were taken on HB1.

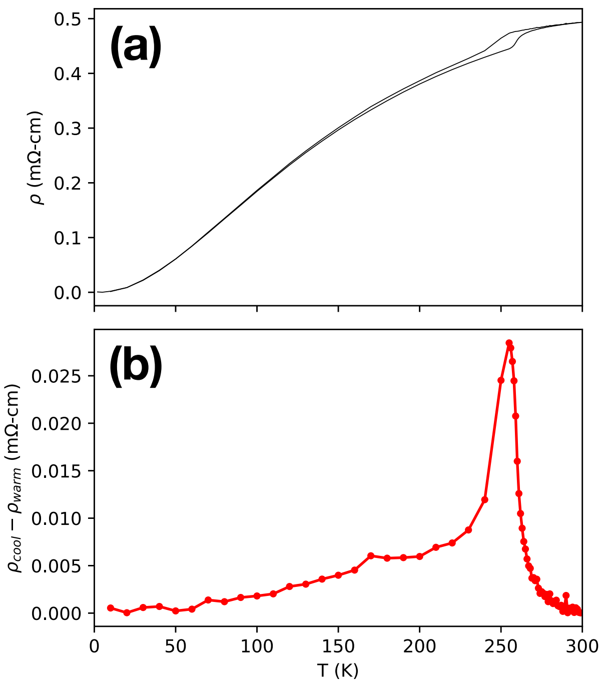


FIG. S4. (a) Resistivity measured on a $MoTe_2$ crystal. Data were taken on cooling from 300 K to 2 K, then warming up to 300 K. (b) Difference between cooling and warming resistivity data in (a).
